# Supplementary material for: Iterative Broadband Source Localization
Source: arXiv:2210.11669 source file (2022-10-21)
Supplement: Supplementary file 1 [file Appendix_CoSaMP_OMP.tex]

\section{CoSaMP and OMP algorithms}
\label{apx:CoSaMP_OMP}
Here we provide a brief overview of the OMP and CoSaMP algorithms adapted to an SLE framework. Pseudo-code for both algorithms are provided in Algorithm~\ref{alg:OMP_SLE} and Algorithm~\ref{alg:CoSaMP_SLE} respectively. The algorithms share several features such as the ``proxy" forming step $\vv = \mPhi^H \vr^{(i)}$, where we examine how well the component signals of $\vy$ align with our model family. Though this is shown as a direct matrix multiplication, since $\mPhi$ is an oversampled Fourier dictionary it can be applied implicitly and efficiently to $\vr$ via an $Nd$-point FFT. The $P_{SLE}(\cdot,\cdot)$ function present in both algorithms estimates the support (e.g. the active frequency bins) of $\vv$ through some version of peak picking. How picking the $L$ most significant peaks is done is somewhat subjective, with sources such as \cite{DUARTE2013111,Fannjiang:2012} utilizing a ``band exclusion" principle while \cite{Davenport:SSCoSaMP} recommends setting $P_{SLE}(\cdot,\cdot)$ to its own sparse approximation sub-routine. The least square nulling step in either algorithm requires a regularization parameter $\gamma$ due to the possibility of highly coherent elements in $\mPhi$ leading $\tilde\mPhi$ to be ill-conditioned. We note that the least squares step can be solved iteratively and efficiently via conjugate gradient descent (CGD) coupled with implicit applications of $\tilde\mPhi$ via FFTs.

The key difference between the two algorithms is that OMP picks one source at a time while CoSaMP produces an overestimation of the support and then ``prunes" this back to $L$ sources. This may be a subtle point but can have substantial implications in terms of performance and analysis, particularly in the case of compressed measurements \cite{Tropp:2010,tropp2007signal}. Therefore it is worth experimentally examining both of these greedy algorithms in the narrowband SLE case as well as the broadband-adapted case.
\begin{center}
\begin{minipage}[t]{0.49 \textwidth}
\vspace{0pt}  
\begin{algorithm}[H]
\caption{OMP for SLE}
\label{alg:OMP_SLE}
\begin{algorithmic}[1]
\State $\vy \gets \vs+\veta$ 
\State $\vr^{(0)} \gets \vy$
\State $\tilde\mPhi^{(0)} \gets \emptyset$
\State $i \gets 0$
\While{Not Converged}
\State $i \gets i+1$
\State $\vv = \mPhi^H\vr^{(i-1)}$
\State $\hat{f}_i \gets P_{SLE}(\vv,1)$
\State $\vphi_i \gets \vphi(\hat{f}_i)$
\State $\tilde\mPhi^{(i)} \gets [\tilde\mPhi^{(i-1)} \, \vphi_i]$ 
\State $\hat\vs \gets \mPhi^{(i)}(\mPhi^{(i)H}\mPhi^{(i)}+\gamma \mtx{I})^{-1}\mPhi^{(i)H}\vy$ 
\State $\vr^{(i)} \gets \vy - \hat\vs $ 
\EndWhile \label{euclidendwhile}
\State $\vf \gets$ frequencies identified in  $\mPhi^{(i)}$
\end{algorithmic}
\end{algorithm}
\end{minipage}%
\hfill
\begin{minipage}[t]{0.49 \textwidth}
\begin{algorithm}[H]
\caption{CoSaMP for SLE}
\label{alg:CoSaMP_SLE}
\begin{algorithmic}[1]
\State $\vy \gets \vs +\veta$, $\vr^{(0)} \leftarrow \vy$,
$\mPhi^{(0)} \leftarrow \emptyset$, $i \leftarrow 0$
\While{Not Converged}
\State $i \gets i+1$
\State $\vv = \mPhi^H\vr^{(i-1)}$
\State $\{ \hat{f}_i \}_{i=1}^{2L} \gets P_{SLE}(\vv,2L)$
\State $\tilde\mPhi_{2L} \gets [\vphi({\hat{f}_1}) \ \cdots \ \vphi({\hat{f}_{2L}}) ]$
\State $\tilde\mPhi^{(i)} \gets [\tilde\mPhi^{(i-1)}\, \tilde\mPhi_{2L}]$ 
\State $\hat\vs \gets \tilde\mPhi^{(i)}(\tilde\mPhi^{(i)H}\tilde\mPhi^{(i)}+\gamma \mtx{I})^{-1}\tilde\mPhi^{(i)}\vy$ 
\State $\{ \hat{f}_i\}_{i=1}^L \gets P_{SLE}(\mPhi^H\hat\vs,L)$
\State $\tilde\mPhi^{(i)} \gets [\vphi(\hat{f}_1) \cdots \ \vphi(\hat{f}_L) ]$
\State $\hat\vs \gets \tilde\mPhi^{(i)}(\tilde\mPhi^{(i)H}\tilde\mPhi^{(i)}+\gamma \mtx{I})^{-1}\tilde\mPhi^{(i)H}\vy$ 
\State $\vr^{(i)} \gets \vy - \hat\vs $ 
\EndWhile \label{euclidendwhile}
 \State $\mtx{f} \gets$ frequencies identified in  $\mtx{\Phi}^{(i)}$
\end{algorithmic}
\end{algorithm}
\end{minipage}
\end{center}
